# Supplementary material for: Simple Ingredients for Offline Reinforcement Learning
Source: arXiv:2403.13097 source file (2024-03-19)
Supplement: Supplementary file 1 [file HExtRes.tex]

\begin{comment}
\section{Extended results}

\label{appH:ext_res}
\end{comment}

\section{Artificial expressivity and scale for offline RL}

\label{appF:details++}
